# Supplementary material for: Re-imagining Algorithmic Fairness in India and Beyond
Source: arXiv:2101.09995 source file (2021-01-27)
Supplement: Supplementary file 1 [file appendix.tex]

%%%%%%%%%%%%%%%%%
%FOR ERIN

\textbf{Glossary}\newline
\begin{table*}
\small
%\centering
\setlength{\tabcolsep}{10pt}
\begin{tabular}{p{1.5in}p{1.5in}}
\toprule
\bf Term & \bf Translation  \\
\midrule
Dalit & xyz \\
Bahujan & xyz \\
Adivasis & xyz \\
Hijra & xyz \\

\bottomrule
\end{tabular}
\normalsize
\caption{Glossary.}
\end{table*}
